# Supplementary material for: Variational structure of Luttinger-Ward formalism and bold diagrammatic expansion for Euclidean lattice field theory
Source: arXiv:1711.07191 ancillary file (2017-11-20)
Supplement: Supplementary file 1 [file supplemental-materials.pdf]

# Supplemental Materials for
# Variational Structure of Luttinger-Ward Formalism and Bold Diagrammatic Expansion for Euclidean Lattice Field Theory


Lin Lin[1,2,*] and Michael Lindsey[1,†]

[1] *Department of Mathematics, University of California, Berkeley, California 94720, United States*

[2] *Computational Research Division, Lawrence Berkeley National Laboratory, Berkeley, California 94720, United States*


*Proof that $\mathcal{F}$ is concave in Theorem 1.* Let $G_1, G_2 \in \mathcal{S}^n_{++}$, $\theta \in [0,1]$, and $\varepsilon > 0$. Note that $\mathcal{F}$ can be written

$$\mathcal{F}[G] = \sup_{\rho \in \mathcal{G}^{-1}(G)} \Psi[\rho], \quad \Psi[\rho] := S(\rho) - \int U\,\rho\,\mathrm{d}x.$$

Furthermore let $\rho_1, \rho_2 \in \mathcal{M}$ such that $\rho_i \in \mathcal{G}^{-1}(G_i)$ and $\Psi[\rho_i] \geq \mathcal{F}[G_i] - \varepsilon/2$. Then, noting that $\theta\rho_1 + (1-\theta)\rho_2 \in \mathcal{G}^{-1}(\theta G_1 + (1-\theta)G_2)$, we observe

$$\begin{aligned}\mathcal{F}[\theta G_1 + (1-\theta)G_2] &= \sup_{\rho \in \mathcal{G}^{-1}(\theta G_1 + (1-\theta)G_2)} \Psi[\rho] \\ &\geq \Psi[\theta\rho_1 + (1-\theta)\rho_2] \\ &\geq \theta\Psi[\rho_1] + (1-\theta)\Psi[\rho_2] \\ &\geq \theta\mathcal{F}[G_1] + (1-\theta)\mathcal{F}[G_2] + \varepsilon,\end{aligned}$$

where the penultimate step employs convexity of $\Psi$. Since $\varepsilon$ was arbitrary, we have established concavity. □

*Proof of the transformation rule (Proposition 4).* Let $G \in \mathcal{S}^n_{++}$. Using $\mathrm{Tr}[\log(G)] = \log\det(G)$, we have

$$\Phi[G;U] = -\Phi_0 - 2 \inf_{\rho \in \mathcal{G}^{-1}(G)} \left[ \int \left( \log\left[ (\det G)^{1/2} \rho \right] + U \right) \rho\,\mathrm{d}x \right].$$

Then for $T$ invertible, we have

$$\Phi[TGT^*;U] = -\Phi_0 - 2 \inf_{\rho \in \mathcal{G}^{-1}(TGT^*)} \left[ \int \left( \log\left[ (\det G)^{1/2} \cdot |\det T| \cdot \rho \right] + U \right) \rho\,\mathrm{d}x \right].$$

Now observe by changing variables that

$$\left\{ \rho \,:\, \rho \in \mathcal{G}^{-1}(TGT^*) \right\} = \left\{ |\det T|^{-1} \cdot \rho \circ T^{-1} \,:\, \rho \in \mathcal{G}^{-1}(G) \right\}.$$

Therefore

$$\begin{aligned}\Phi[TGT^*;U] &= -\Phi_0 - 2 \inf_{\rho \in \mathcal{G}^{-1}(G)} \left[ |\det T|^{-1} \int \left( \log\left[ (\det G)^{1/2} \cdot \rho \circ T^{-1} \right] + U \right) \rho \circ T^{-1}\,\mathrm{d}x \right] \\ &= -\Phi_0 - 2 \inf_{\rho \in \mathcal{G}^{-1}(G)} \left[ \int \left( \log\left[ (\det G)^{1/2} \cdot \rho \right] + U \circ T \right) \rho\,\mathrm{d}x \right] \\ &= \Phi[G; U \circ T],\end{aligned}$$

as was to be shown. □

*Proof of Lemma 5.* Write

$$\begin{aligned}x^T A x + U(x) &= x^T \left( A - \Sigma(\varepsilon) + \overline{\Sigma}^{(N)}(\varepsilon) \right) x + U^{(N)}_\varepsilon(x) \\ &= x^T \left( G^{-1} + \overline{\Sigma}^{(N)}(\varepsilon) \right) x + U^{(N)}_\varepsilon(x).\end{aligned}$$

It follows that under the interaction $U_\varepsilon^{(N)}$, the non-interacting Green's function $G^{-1} + \overline{\Sigma}^{(N)}(\varepsilon)$ corresponds to the interacting Green's function $G$. This establishes that

$$A[G; U_\varepsilon^{(N)}] = G^{-1} + \overline{\Sigma}^{(N)}(\varepsilon).$$

Moreover, by the Dyson equation we have that

$$\Sigma[G; U_\varepsilon^{(N)}] = A[G; U_\varepsilon^{(N)}] - G^{-1} = \overline{\Sigma}^{(N)}(\varepsilon),$$

as desired. □

*Proof of the expansion coefficients of the LW functional in Theorem 3.* By the transformation rule (and the fact that $U$ is quartic), we have

$$\Phi[tG, \varepsilon U] = \Phi[G, t^2 \varepsilon U]$$

for any $G \in \mathcal{S}_{++}^n$ and $\varepsilon, t > 0$. Taking the gradient in $G$ of both sides yields

$$\Sigma[tG, \varepsilon U] = \frac{1}{t} \Sigma[G, t^2 \varepsilon U].$$

Then compute:

$$\begin{aligned}
\Phi[G, \varepsilon U] &= \int_0^1 \frac{d}{dt} \Phi[tG, \varepsilon U]\, dt \\
&= \int_0^1 \operatorname{Tr}[G \Sigma[tG, \varepsilon U]]\, dt \\
&= \int_0^1 \frac{1}{t} \operatorname{Tr}[G \Sigma[G, t^2 \varepsilon U]]\, dt \\
&= \int_0^1 \frac{1}{t} \left[ \sum_{k=1}^N \operatorname{Tr}\left[ G \Sigma_G^{(k)} \right] t^{2k} \varepsilon^k + O\left( t^{2(N+1)} \varepsilon^{N+1} \right) \right] dt \\
&= \int_0^1 \left[ \sum_{k=1}^N \operatorname{Tr}\left[ G \Sigma_G^{(k)} \right] t^{2k-1} \varepsilon^k + O\left( t^{2N+1} \varepsilon^{N+1} \right) \right] dt.
\end{aligned}$$

Now since $t$ ranges from 0 to 1 in the integrand, we have that $t^{2N+1}\varepsilon^{N+1} \le \varepsilon^{N+1}$, and therefore

$$\begin{aligned}
\Phi[G; \varepsilon U] &= \int_0^1 \left[ \sum_{k=1}^N \operatorname{Tr}\left[ G \Sigma_G^{(k)} \right] t^{2k-1} \varepsilon^k \right] dt + O(\varepsilon^{N+1}) \\
&= \sum_{k=1}^N \frac{1}{2k} \operatorname{Tr}\left[ G \Sigma_G^{(k)} \right] \varepsilon^k + O(\varepsilon^{N+1}).
\end{aligned}$$

This establishes that

$$\Phi_G^{(k)} = \frac{1}{2k} \operatorname{Tr}\left[ G \Sigma_G^{(k)} \right],$$

as was to be shown.

We remark that this proof bears resemblance to the adiabatic integration technique that formally defines the LW functional [1, 2]. The significant difference lies in the fact that in our case, the adiabatic integration technique is used to establish the relation of the coefficients for the LW functional that we have *already defined.* Moreover, unlike the diagrammatic constructions of the LW functional, our argument does not make use of any particular properties of the bold diagrams, relying instead on the transformation rule. □

* linlin@math.berkeley.edu
† lindsey@math.berkeley.edu

[1] J. M. Luttinger and J. C. Ward, Phys. Rev. **118**, 1417 (1960).
[2] R. M. Martin, L. Reining, and D. M. Ceperley, *Interacting Electrons* (Cambridge Univ. Pr., 2016).
